# Supplementary material for: MMVP: Motion-Matrix-based Video Prediction
Source: arXiv:2308.16154 source file (2023-08-31)
Supplement: Supplementary file 1 [file 1-Implementation.tex]

\section{Framework Implementation}
This section we demonstrate the inner structure of each module that we adopted for MMVP implementation in this work. MMVP contains three major steps: i) feature extraction, which includes an image encoder and a filter block, see Figure~\ref{fig:step1}; ii) motion matrix construction and prediction, see Figure~\ref{fig:step2}; and iii) Future composition and decoding, see Figure~\ref{fig:step3}. We will apply a softmax operation to every $\mathbf{M}$ before they take part in the future composition step.
\begin{figure}[tbh!]
    \centering
    \includegraphics[width=0.5\textwidth]{iccv2023AuthorKit/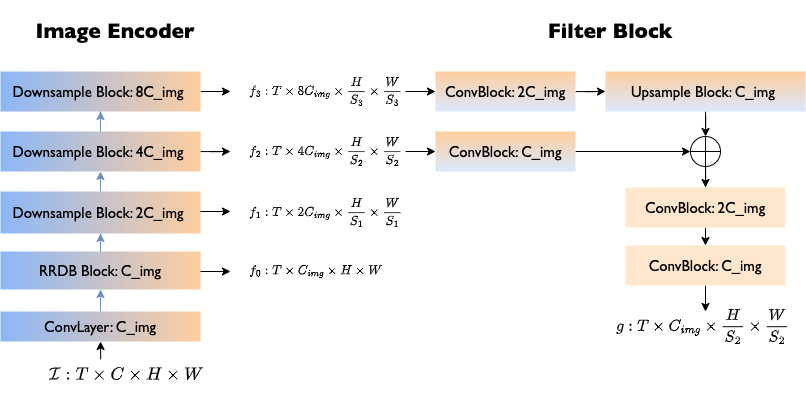}
    \caption{Spatial feature extraction.}
    \label{fig:step1}
\end{figure}

\begin{figure}[tbh!]
    \centering
    \includegraphics[width=0.5\textwidth]{iccv2023AuthorKit/figures/matrix_construction_prediction.png}
    \caption{Motion matrix construction and prediction.}
    \label{fig:step2}
\end{figure}

\begin{figure}[tbh!]
    \centering
    \includegraphics[width=0.5\textwidth]{iccv2023AuthorKit/figures/composition_decoding.png}
    \caption{Future composition and decoding.}
    \label{fig:step3}
\end{figure}

For the experiments on each dataset, the implementations all follow the structures shown in Figure ~\ref{fig:step1},~\ref{fig:step2}, and  ~\ref{fig:step3}. However, there are three hyperparameters that are different when implementing the models for different datasets: i) $C_{img}$, the base channel of the image encoder \& decoder; ii) $C_{motion}$, the base channel of the matrix predictor and iii) the down-sample ratio $S$ between the hidden features and the original image. When selecting the two base channel numbers, we consider the video resolution, the complexity of the motion patterns, and the length of the future frames. For most cases, when video resolution is higher, or the images are more informative, $C$ should be set to a larger number; when the motion pattern is more complex or the prediction length is longer, $C_{motion}$ should be larger. Here we show the $C_{img}$ and $C_{motion}$ for each dataset in Tab. \ref{tab:hyper}. Interestingly, it is easy to note that the model we use on Moving-MNIST consists of the largest parameter numbers among the three datasets while Moving-MNIST is a single channel image with only digit numbers. One reason is that the motion pattern of Moving-MNIST has the least constraints among the three, the two digits are bouncing everywhere on the image, which requires the model to have a larger capacity. 
We will release the code and the pre-trained models later. In MMVP paper, we choose not to exhaustively search for the optimal combination of the hyper-parameters for each dataset setting or the best network architecture for the image encoder, decoder, and matrix predictor. One may modify our code and achieve better results than what we showcase in the paper. 

\begin{table}[tbh!]
    \centering
    
    \scalebox{0.8}{
    
    \begin{tabular}{c|cccccc}
    \toprule
         Dataset&   Resolution  & Future length &    $C_{img}$   &   $C_{motion}$  &   $S$ &   Param \# \\
         \hline
         \hline
         UCF Sports&    $512\times 512$   &   1   &   32  &   8  &   8  &   2.8M   \\ 
         KTH&    $128\times 128$   &   20   &   16  &   96  &   4 &   4.5M  \\ 
         KTH&    $128\times 128$   &   40   &   16  &   96  &   4 &   6.1M  \\
         MNIST&    $64\times 64$   &   10   &   32  &   192   &   4    &   14.6M   \\ 
         \toprule
    \end{tabular}
    }
    \caption{Hyper-parameters in the MMVP implementation for different datasets.}
    \label{tab:hyper}
\end{table}

When running the experiments on our splits of UCF sports dataset using SimVP\cite{gao2022simvp} and STIP\cite{chang2022stip}, we strictly follow the hyper-parameters released in their official code. Especially, for STIP, we directly copy their hyper-parameters on the UCF Sports dataset.
