# Supplementary material for: MMVP: Motion-Matrix-based Video Prediction
Source: arXiv:2308.16154 source file (2023-08-31)
Supplement: Supplementary file 2 [file 2-dataset.tex]

\section{Extensive Visualization}
\subsection{UCF Sports Validation subset}
In the paper, we have mentioned that we notice that even within the same validation set, the difficulty level of different samples varies a lot. Some video clips only contain static backgrounds and slow-moving objects while others include drastic camera movement or fast-moving objects. To better understand the model's prediction ability for different scenarios, we use certain thresholds of the structural similarity index measure (SSIM) between the last observed frame and the first future frame to divide the UCF Sports validation set into three subsets: the easy (SSIM $\leq$ 0.9), intermediate, hard subsets (SSIM $<$ 0.6),
which take 66\%, 26\%, and 8\% of the full set respectively. 

Here we showcase two examples from each subset in Figure~\ref{fig:dataset}. We can see that for the samples belonging to the easy subset, the difference between the last observed frame $I_T$ and the first future frame $I_{T+1}$ is very minor, which turns the video prediction task into a signal processing or image reconstruction task (especially for the second sample). Methods that rely too much on the feature shortcuts from the previous methods will have leading performances. Comparing the second sample in the intermediate subset and the first sample in the hard subset, we can clearly observe that the sample in the hard subset may contain more camera movement, which is more challenging for the video prediction system.  

\begin{figure*}[tbh!]
    \centering
    \includegraphics[width=0.98\textwidth]{iccv2023AuthorKit/figures/dataset_sample.png}
    \caption{Samples from different subsets of the validation set in UCF Sports. The last column is the overlay of the last observed frame $I_T$ and the first future frame $I_{T+1}$.}
    \label{fig:dataset}
\end{figure*}
\subsection{Motion Matrix Sequence}
In this section, we visualize the motion sequences that are input to the matrix predictor and their corresponding output (See Figure~\ref{fig:matix_seq}). Specifically, in KTH, we demonstrate what the output will be like if it is a sequence of matrices. From the visualization we have two observations: i) For long-term prediction in KTH, the highlighted area of the selected matrix can still fall in the correct region; ii) the heatmap of the matrix describes the layout of each frame, and the basic shapes of the objects in the video. Furthermore, it can be regarded as a semantic segmentation map while the sequence of the matrices reflects the changing pattern of the semantic meaning. All those information provides essential hints for motion prediction.

\begin{figure*}
\centering
    \includegraphics[width=0.95\textwidth]{iccv2023AuthorKit/figures/matrix_seq.png}
    
    \caption{Visualization of the motion matrices. We selected one patch for each video sequence at $(h,w)$ and visualize its corresponding sequence of the matrices as well as the predicted matrices output by the matrix predictor. The selected patch is red in the UCF Sports data sample and white in the KTH data sample. }
    \label{fig:matix_seq}
\end{figure*}

\subsection{Extra Qualitative Results} 

In this section, we show the qualitative results for the other two datasets: Moving-MNIST~(Fig. \ref{fig:mnist}) and KTH~(Fig. \ref{fig:kth}

\begin{figure*}
    \centering
    \includegraphics[width=0.8\textwidth]{iccv2023AuthorKit/figures/MNISTtrain_3000.png}
    \caption{Qualitative results for Moving-MNIST. The upper row of each sample shows the ground truth for 10 future frames and the lower row is the output of MMVP.}
    \label{fig:mnist}
\end{figure*}

\begin{figure*}
    \centering
    \includegraphics[width=1\textwidth]{figures/kth.png}
    \caption{Qualitative results for KTH. The upper row of each sample shows the ground truth for 20 future frames and the lower row is the output of MMVP.}
    \label{fig:kth}
\end{figure*}
