# Supplementary material for: MMVP: Motion-Matrix-based Video Prediction
Source: arXiv:2308.16154 source file (2023-08-31)
Supplement: Supplementary file 3 [file 0-training.tex]

\section{Training strategy}
All models in the paper are implemented using Pytorch\cite{paszke2019pytorch} on a single NVIDIA A100 GPU. The initial learning is set to be $1e^{-3}$ and decayed following a cosine restart learning scheduler\cite{loshchilov2016sgdr}. We use AdamW optimizer during the training. We show the other training-related hyperparameters for each dataset in Table \ref{tab:training_param}.

\begin{table}[tbh!]
    \centering
    \scalebox{0.8}{
    \begin{tabular}{c|cccc}
    \toprule
      Dataset   &   Restart Period &   Batch Size    &   Total Epoch  \\
      \hline
      \hline
      UCF Sports   &    100  &   4   &   300   \\
      KTH   &    50  &   16   &   150   \\
      MNIST  &    1000  &   32   &   3000   \\
      \toprule
    \end{tabular}
    }
    \caption{Training configuration for each dataset in the paper.  }
    \label{tab:training_param}
\end{table}
